# Supplementary material for: Learning More Expressive General Policies for Classical Planning Domains
Source: arXiv:2403.11734 source file (2025-02-18)
Supplement: Supplementary file 1 [file appendix.tex]

\clearpage
\appendix

\section*{Technical Appendix}

This appendix provides additional details and analysis that supplement the main content of our paper.
The first part explains the domains used in our experiments, including a description of the parameters used in both the training and test sets.
The second part offers an analysis of the domains that require $C_3$ logics, explaining why $C_2$ is insufficient to generalize properly.

\input{sections/domains.tex}

\subsection*{Analysis for C$_3$ Domains}

We will now take a closer look at the $C_3$ domains and explain why $C_2$ cannot achieve generalization.

\paragraph{Grid.}

In the Grid domain, the objective is to go to a specific cell on a grid.
However, access to this cell is obstructed by locked doors, each requiring a key of a specific shape.
Moreover, one locked door may be behind another, creating a sequence of barriers.
The placement of keys within the rooms is such that it ensures the overall instance is solvable.

This domain includes, among others, the binary predicates $\textsc{Key-Shape}/2$ and $\textsc{Lock-Shape}/2$.
For example, consider a key $k$ with shape $s$, as denoted by $\textsc{Key-Shape}(k, s)$, and a lock $l$, also with shape $s$, indicated by $\textsc{Lock-Shape}(l, s)$.
In this case, they match, allowing the key to be used to open the lock.
We believe that this domain requires $C_3$ expressiveness, as the feature $\textsc{Can-Unlock}(k, l)$, indicating that $k$ can open $l$, is likely a necessary composition (which requires $C_3$).
Additionally, this feature should be associated with and "stored" in the embedding for the pair $\langle k, l \rangle$.
It cannot be associated solely with $k$, as there are an arbitrary number of locks, nor can it be associated with $l$ for the same reason.
Thus, with an embedding for every pair, the capacity for storing the required features scales appropriately with the number of objects.

We believe these observations explain our experimental results: \extended{$0$} outperforms B because it can appropriately store an approximation of the composition.
Similarly, \extended{$1$} outperforms \extended{$0$} by actually computing the composition instead of approximating it.
Nonetheless, we did not achieve $100 \%$ coverage.
Upon inspecting the $5$ unsolved instances, we observed that the lengths of the \emph{optimal} plans varied between 25 and 44 steps.
As noted by~\cite{stahlberg-et-al-icaps2022}, the network's capability to compute distances is bounded by the number of layers.
The plans primarily involve moving to specific cells to collect keys and unlock doors.
In our experiments, we used $30$ layers, and the lengths of the optimal plans likely exceeded the network's reasoning capacity (rather than expressive capacity).
We note that, when a plan is found, it tends to be near-optimal.
The mean and median values for optimal plans of the solved instances are both $13$, mirroring those for \extended{$1$}.

\paragraph{Logistics.}

In Logistics, as noted by~\cite{stahlberg-et-al-kr2022,stahlberg-et-al-kr2023}, the delivery of multiple packages requires $C_3$ expressiveness to determine if an airplane is in the correct city for a package in its cargo.
In their experiments, they achieved $100 \%$ coverage by introducing \emph{derived predicates}, which are defined by \emph{composing} binary relations.
More specifically, in~\cite{stahlberg-et-al-kr2022}, they provided derived predicates for the compositions: $\textsc{At} \circ \textsc{In-City}$, $\textsc{At}_g \circ \textsc{In-City}$, $\textsc{In} \circ \textsc{At}$, and $\textsc{In} \circ \textsc{At} \circ \textsc{In-City}$.
The hyperparameter $t$ in R-GNN[$t$], corresponds to the number of compositions performed recursively through the new ternary predicate.
In our experiments, it seems that only one composition is needed to learn a value function, while they used two.
We emphasize that our compositions were learned automatically, in contrast to their handcrafted approach, which is a significant difference.

\paragraph{Vacuum.}

Vacuum is a simplified version of Rovers, and was designed to illustrate that $C_2$ expressiveness is insufficient for learning an optimal value function for Rovers~\cite{stahlberg-et-al-icaps2022}.
The domain has a ternary predicate $\textsc{Adjacent}(r, x, y)$, signifying that robot $r$ can move from location $x$ to location $y$ in a single action.
Each robot operates within its unique traversal map, and the objective is to clean a specific dirty location $g$.
The optimal value function involves computing the distance from each robot's current location to $g$ and directing the nearest robot towards $g$.
While the baseline achieved $100 \%$ coverage, it did so with excessively long plan lengths.
This suggests that the model struggles to reliably identify good successor states, and it seems more coincidental than intentional when the model directs a robot to the goal location that requires cleaning.

The existence of a path of length $k$ from a robot $r$ at a location $x$ to the dirty goal location is defined by the equations:
\begin{align}
    \textsc{P}_0(r, x) &= \textsc{Dirty}(x) \notag \\
    \textsc{P}_k(r, x) &= \exists y \left[ \textsc{Adjacent}(r, x, y) \wedge \textsc{P}_{k -1}(r, y) \right] \notag
\end{align}
Here, we need three variables in the second equation, placing it in $C_3$.
For the baseline, a practical limitation arises from the inability to store computed distances from a location $x$ to $g$ for robot $r$.
We need to store not only the final distance, but also intermediate distances to compute the final value.
However, storing these distances in the embedding for each robot is problematic due to an arbitrary number of locations.
Similarly, storing distances in the embedding for each location is also not possible due to an arbitrary number of robots.
In contrast, the other methods can store the distances at the robot-location pair $\langle r, x \rangle$.
Furthermore, this pair, together with $\langle r, y \rangle$, are specifically referenced in the extended predicate of $\textsc{Adjacent}$.
This extended predicate and the pair embeddings are sufficient to compute all shortest paths, and we believe this explains the performance difference between the baseline and extended versions.

\paragraph{Rovers.}

Vacuum is essentially a subproblem of Rovers.
Each rover operates within its own traversal map, defined by the predicate $\textsc{Can-Traverse}/3$, necessitating at least $C_3$ expressiveness.
However, after data collection, it must also be wirelessly communicated back to the lander, provided the lander is visible from the current location.
That is, the existence of a path with total length $k_1 + k_2$ from a rover $r$ at location $x$ to a point of interest (POI), where an action is performed, and then back to a location for data transmission, is expressed as:
\begin{align}
\textsc{P}^1_{0,k_2}(r, x) &= \left[ \textsc{POI}(x) \vee \textsc{Has-Sample}(r) \right] \wedge \textsc{P}^2_{k_2}(r, x) \notag \\
\textsc{P}^1_{k_1, k_2}(r, x) &= \exists y \left[ \textsc{Can-Trav.}(r, x, y) \wedge \textsc{P}_{k-1, k_2}(r, y) \right] \notag \\
\textsc{P}^2_{0}(r, x) &= \exists y \left[ \textsc{Lander-Loc.}(y) \wedge \textsc{Visible}(x, y) \right] \notag \\
\textsc{P}^2_{k_2}(r, x) &= \exists y \left[ \textsc{Can-Trav.}(r, x, y) \wedge \textsc{P}^2_{k_2-1}(r, y) \right] \notag
\end{align}
Note that in the base case for the first path, $\textsc{P}^1$, there are two criteria: the point of interest, or if the rover already has the sample.
In the latter case, the rover, having visited the POI and performed the necessary action, only needs to reach a location for data transmission to the lander.
If predicates not part of the state, i.e., $\textsc{POI}$, $\textsc{Has-Sample}$, and $\textsc{Lander-Location}$, fall within $C_3$, then this subproblem also remains in $C_3$.

Rovers may need to sample at most $3$ POIs.
Given the fixed number of POIs, it is possible to derive equations that follow the same pattern, dividing the path into up to $4$ segments.
This feature is quite complex and presents a challenging optimization problem: directing rovers to minimize the total length of the plan.
To test whether the poor quality of plans is due to the optimization problem, we tried a version with just one rover.
This resulted in $95 \%$ coverage with plans that were very close to optimal.
Therefore, we believe the difficulty for the model lies in addressing the optimization problem, not in the complexity of the feature itself.

\paragraph{Visitall-xy.}

We provided an example of a similar domain earlier. The key difference in this
domain is the absence of obstacles, with the added goal of visiting multiple
locations. Nevertheless, we believe that the analysis for this example is also
applicable here. Specifically, for $t \geq 1$, the $\join$ relation allows for
direct communication between adjacent cells.
